# Supplementary material for: SGFormer: Satellite-Ground Fusion for 3D Semantic Scene Completion
Source: arXiv:2503.16825 source file (2025-04-10)
Supplement: Supplementary file 1 [file X_suppl.tex]

\clearpage
\setcounter{page}{1}
\maketitlesupplementary
\begin{figure}
    \centering
    \includegraphics[width=\linewidth]{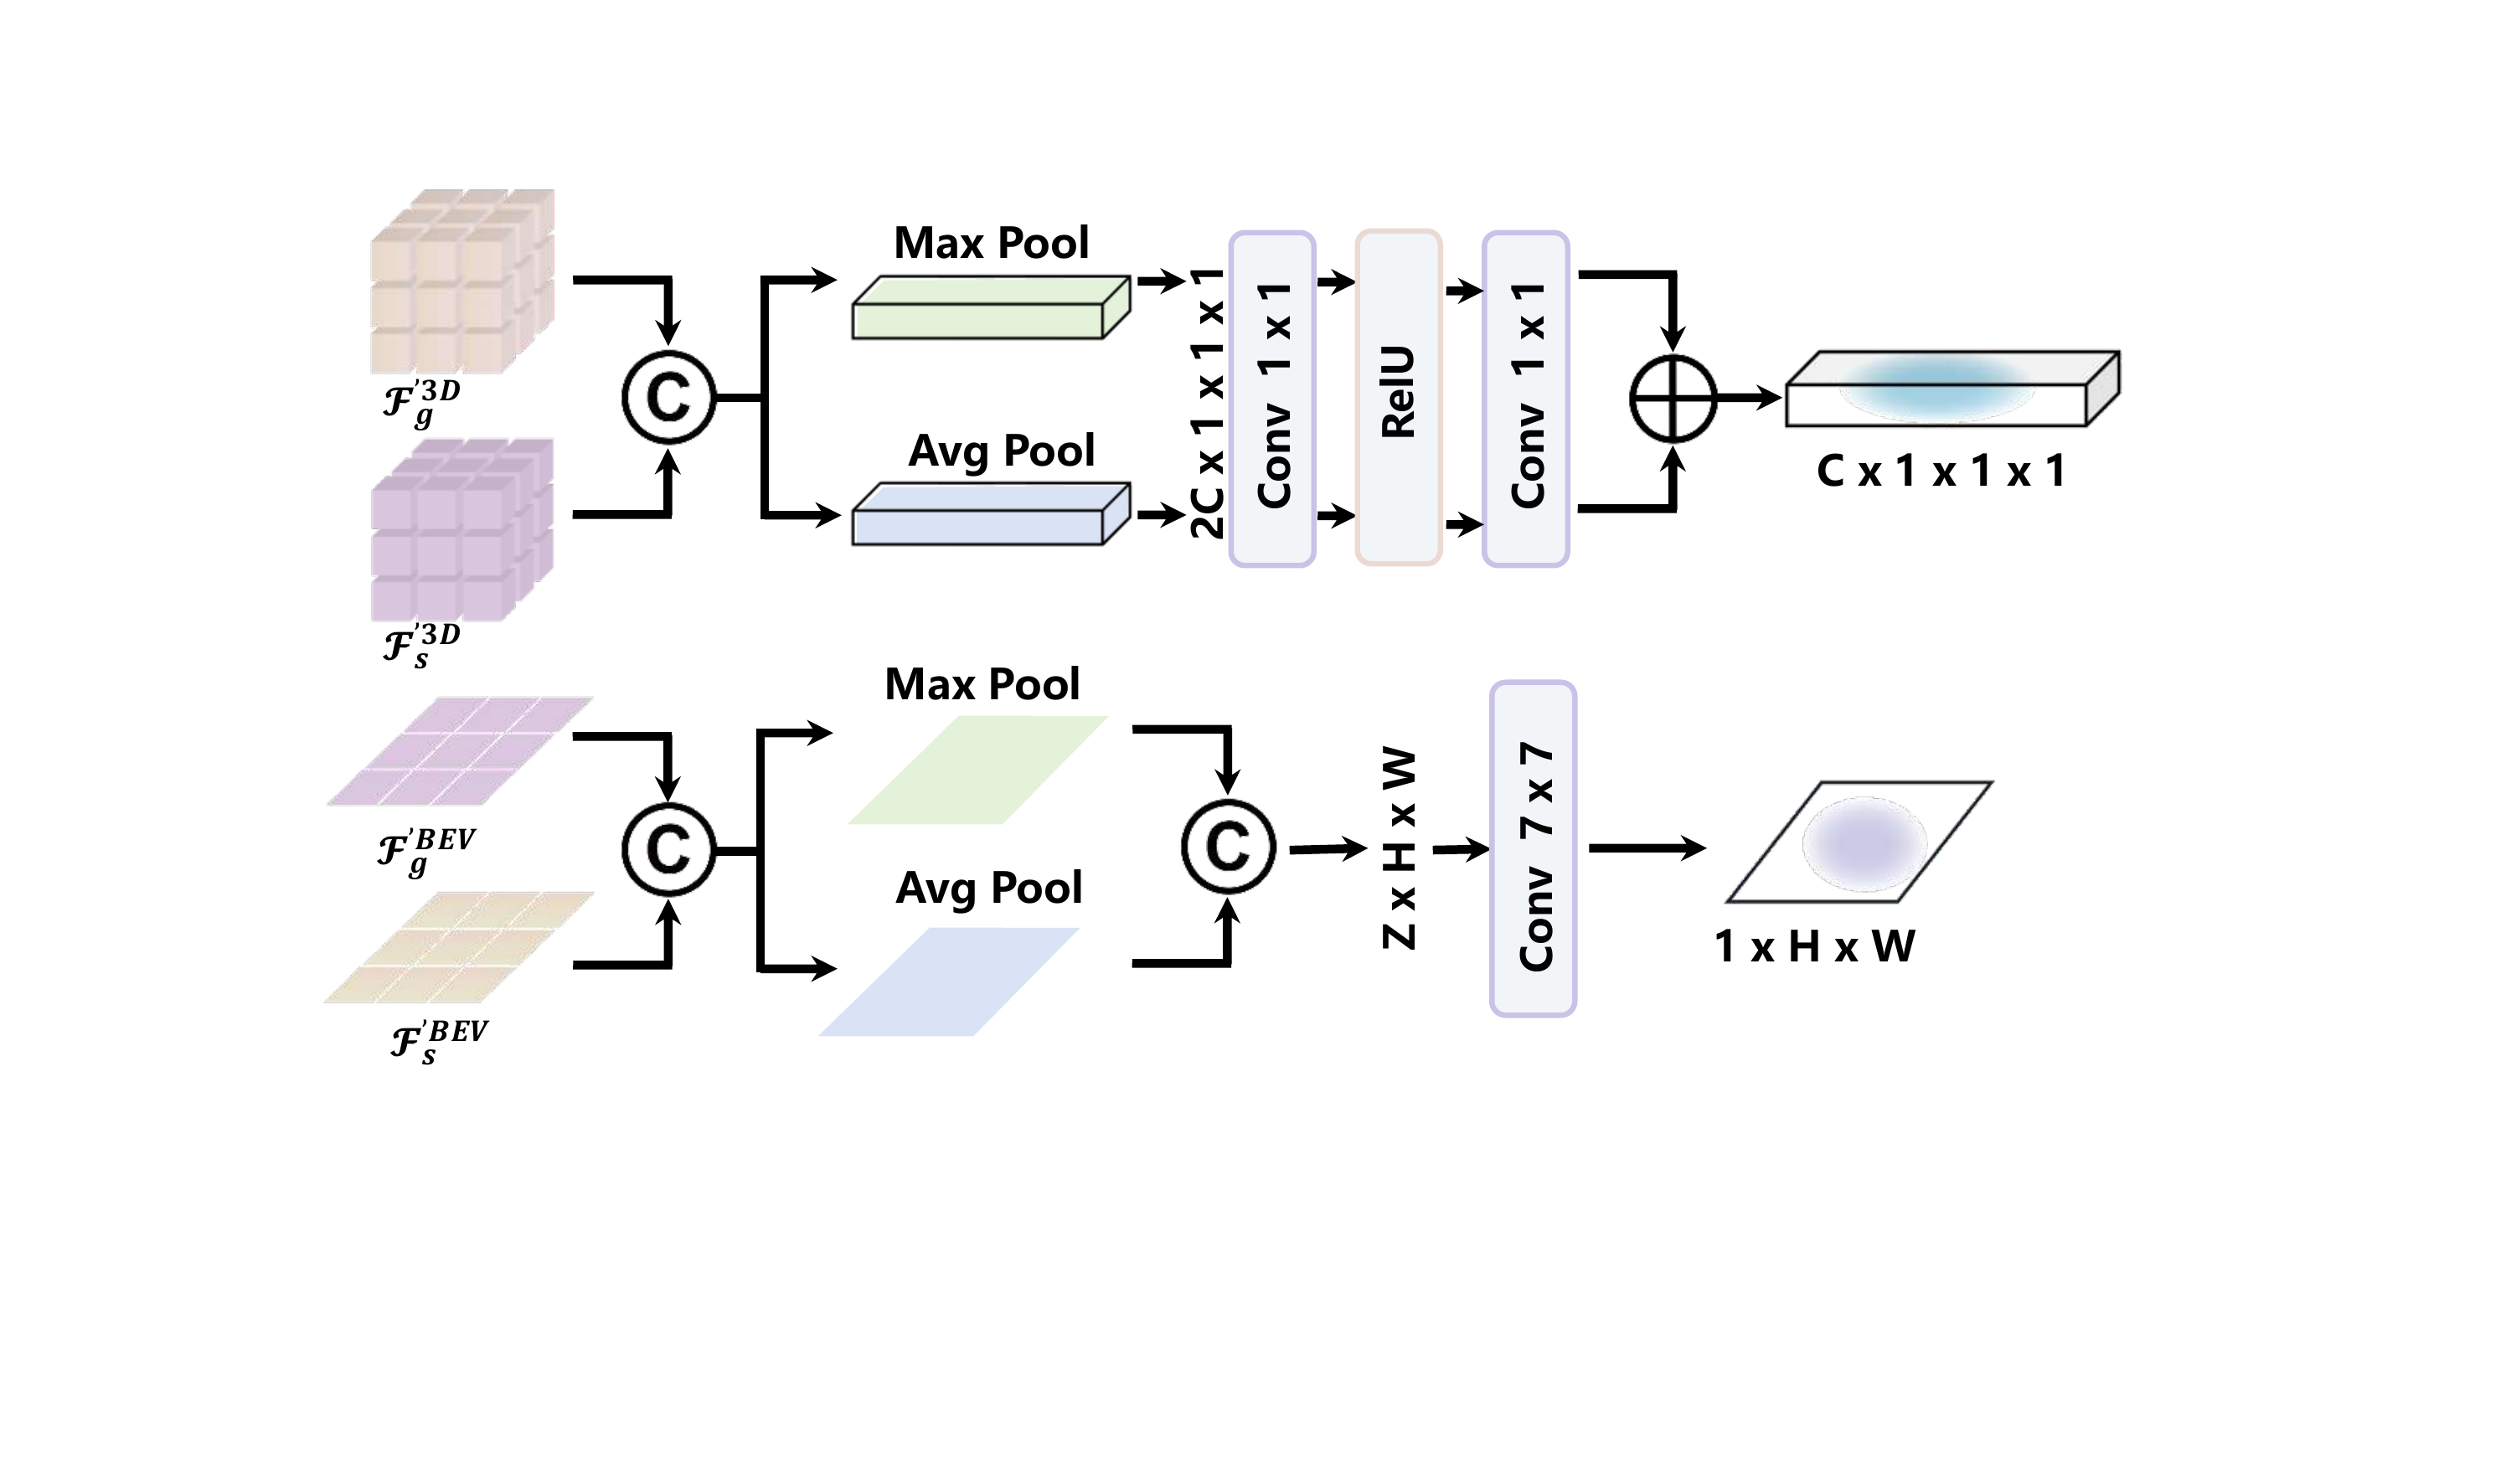}
    \caption{\textbf{Channel and Spatial Attention.}Our channel attention mechanism (\textbf{top part}) utilizes average and maximum pooling operations, followed by shared MLP layers. Similarly, our spatial attention mechanism (\textbf{bottom part}) employs the same pooling operations, paired with $7 \times 7$ convolution layer.}
    \label{fig:attention}
\end{figure}
\begin{figure*}[tb]
    \centering
  \begin{subfigure}{0.33\linewidth}
    \includegraphics[width = \linewidth]{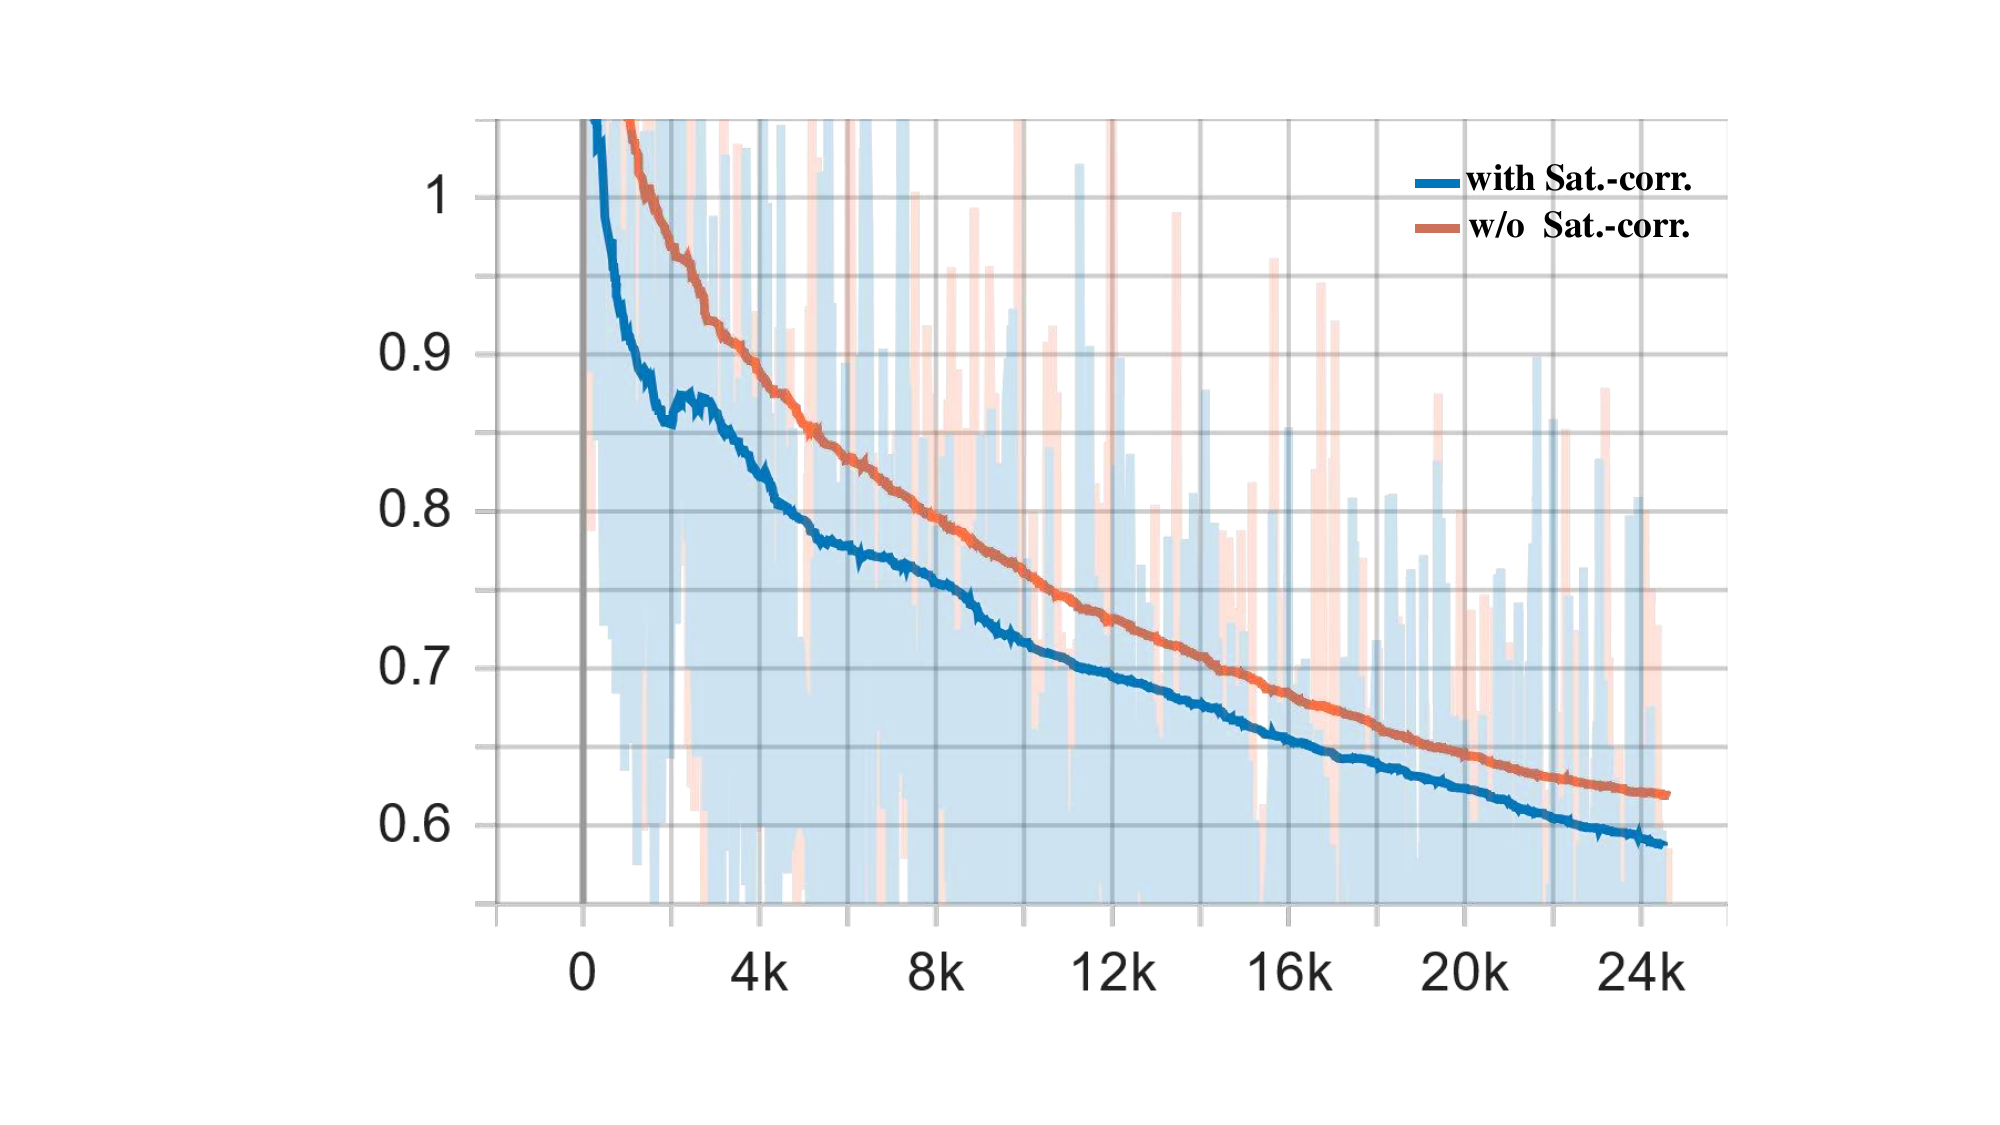}
    \caption{BEV loss curve.}
    \label{fig:bev_loss}
  \end{subfigure}
    \begin{subfigure}{0.33\linewidth}
    \includegraphics[width = \linewidth]{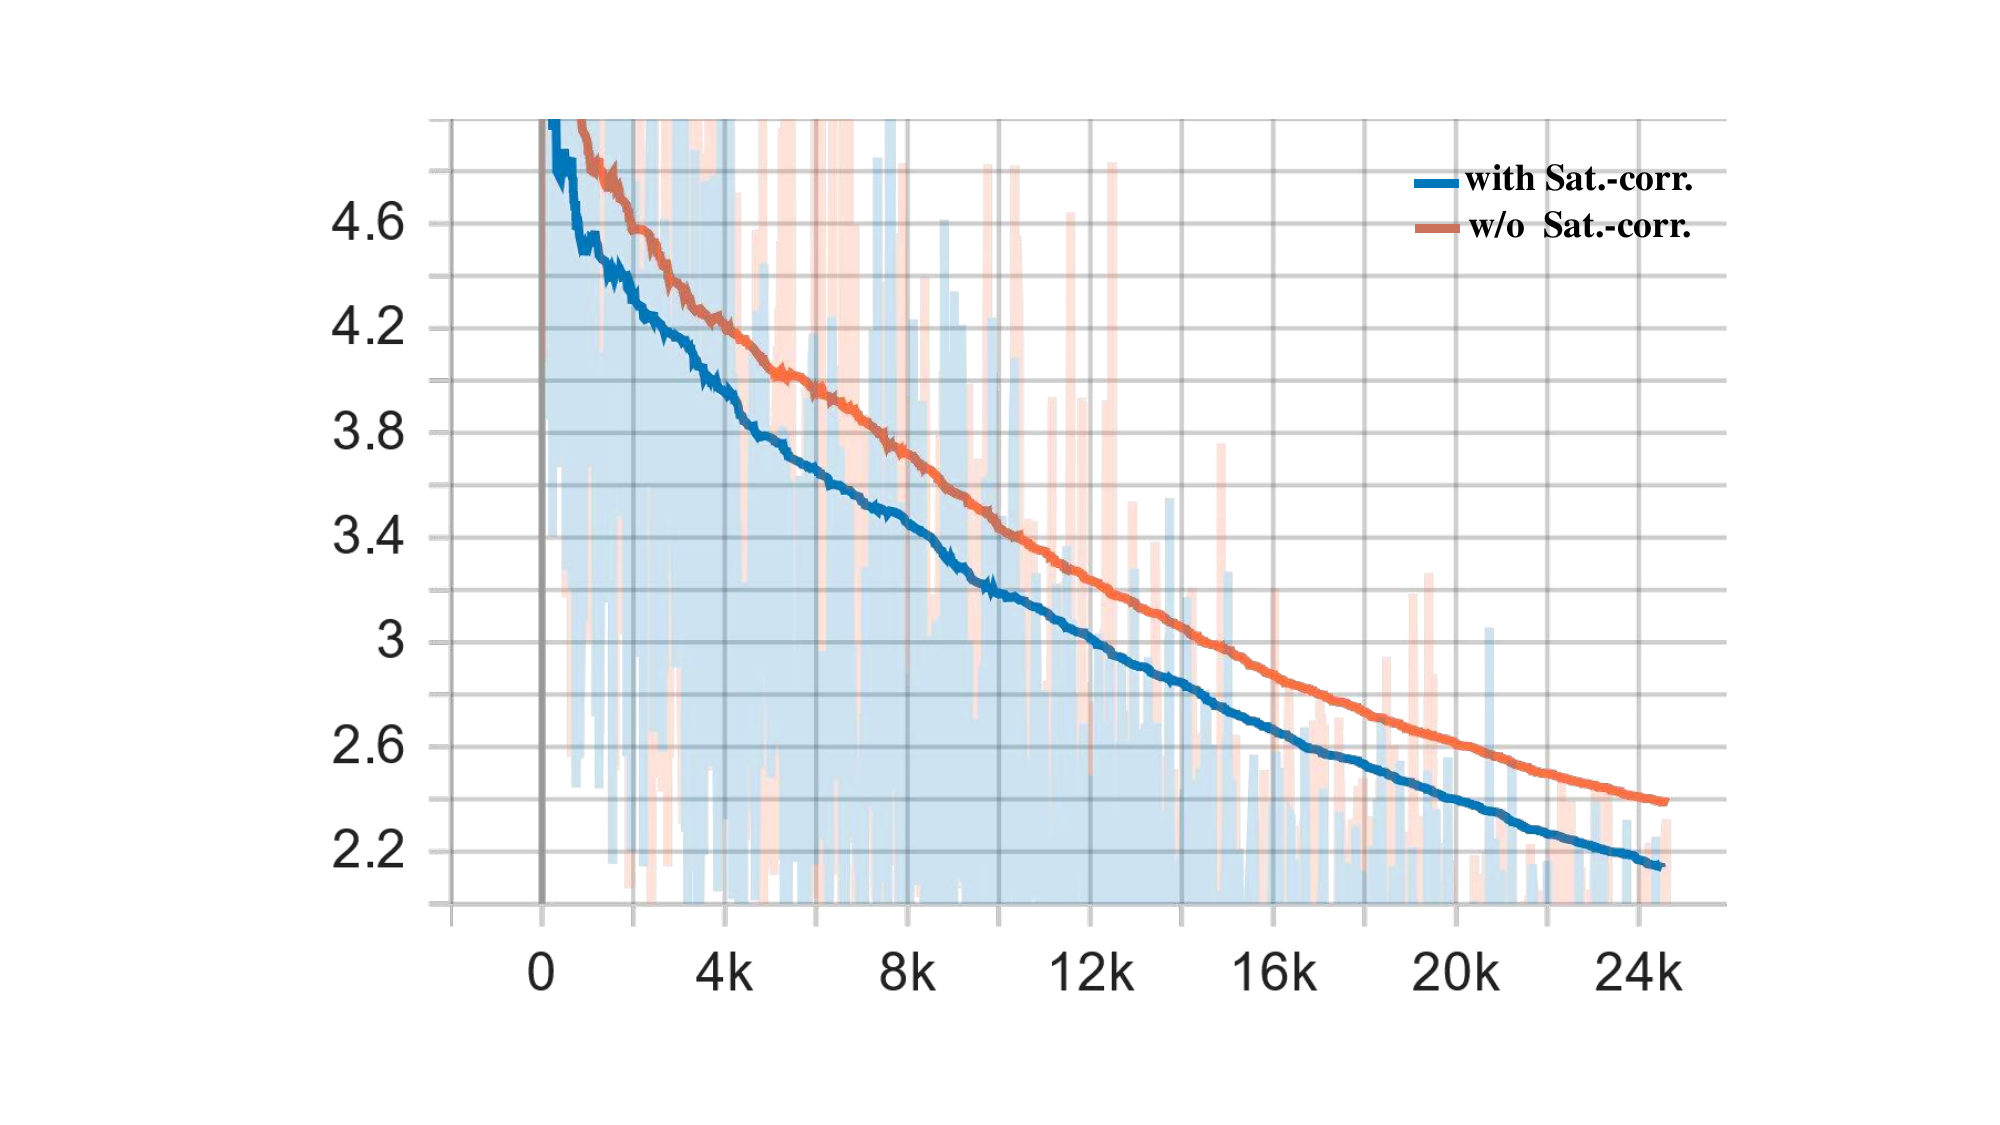}
    \caption{ Scene class affinity loss curve.}
    \label{fig:Affinity_loss}
  \end{subfigure}
  \begin{subfigure}{0.33\linewidth}
    \includegraphics[width = \linewidth]{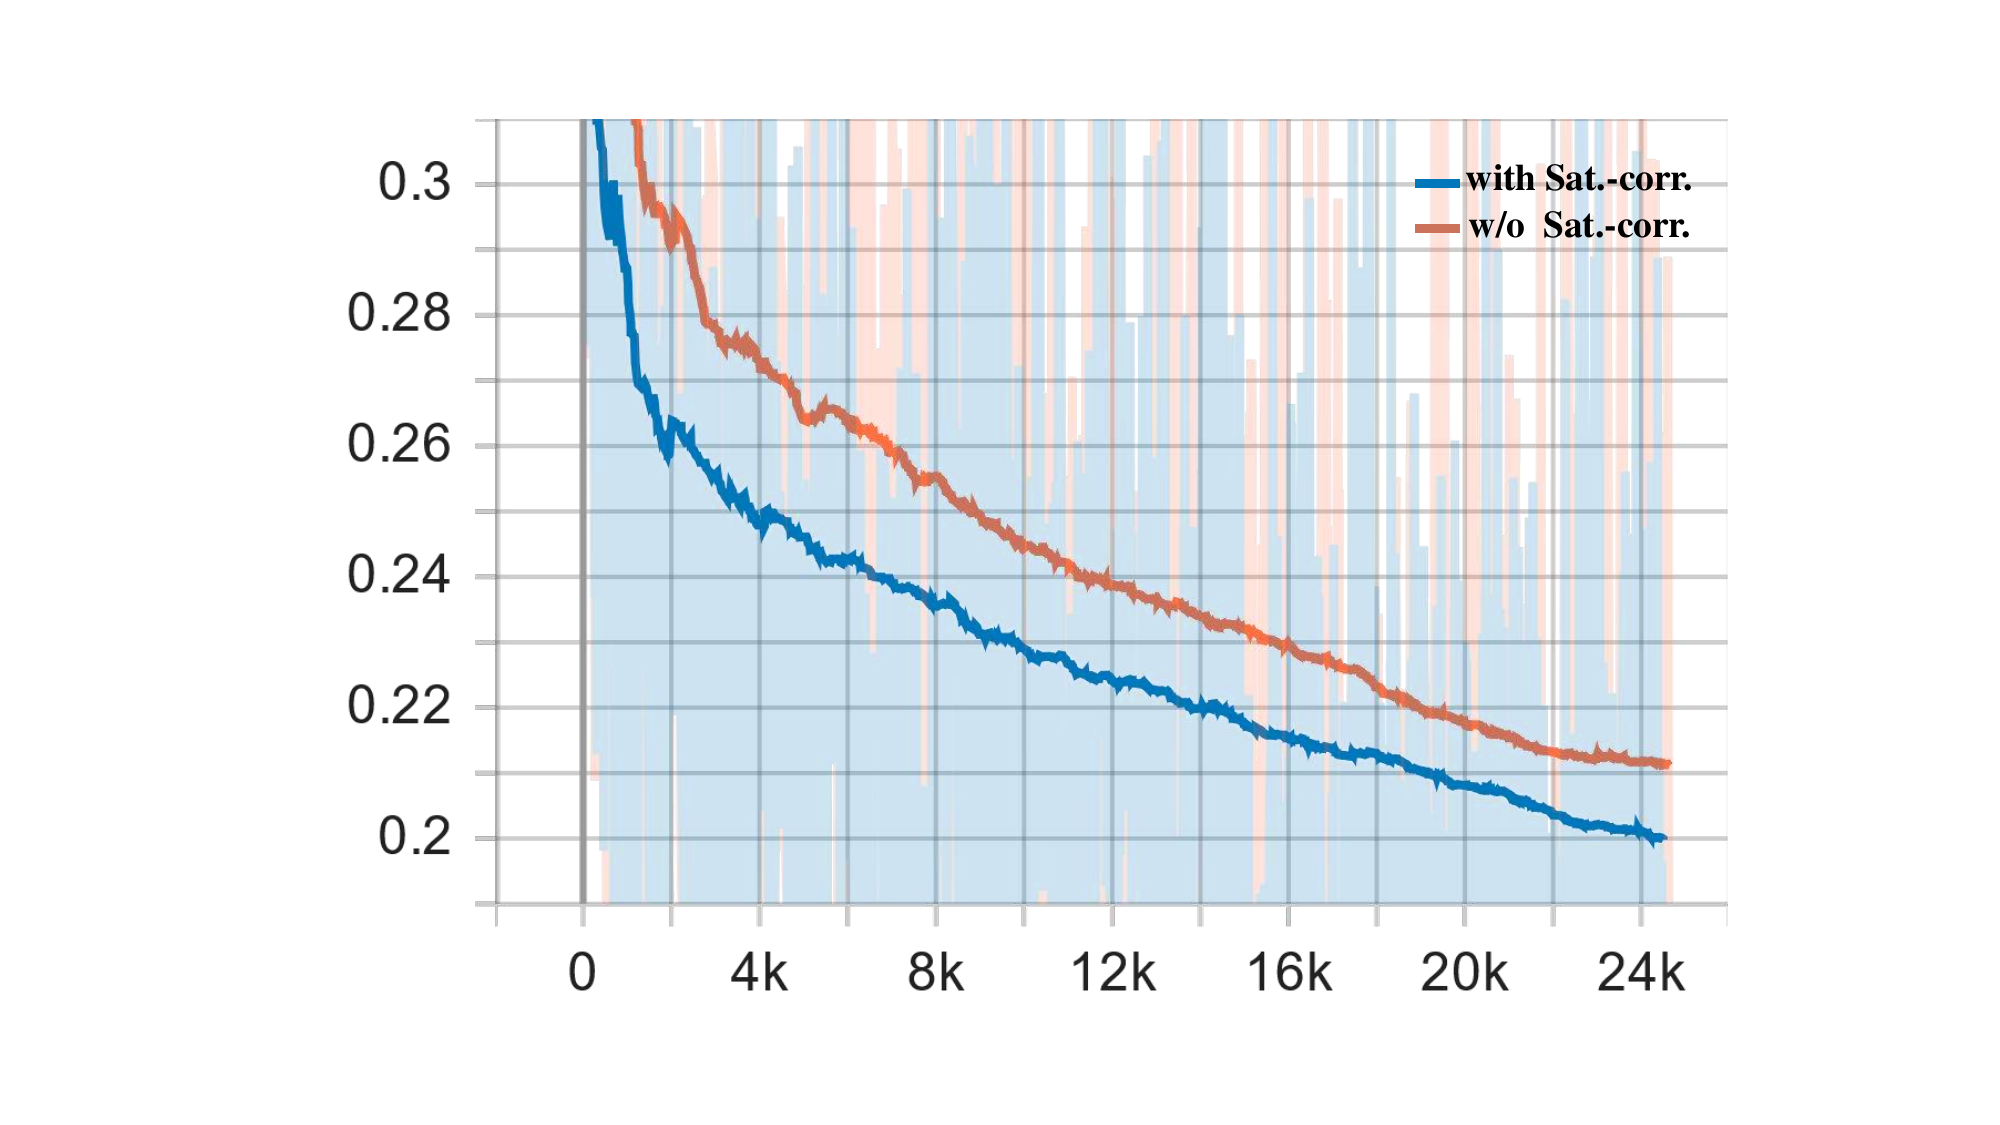}
    \caption{Cross-entropy loss curve.}
    \label{fig:entrop_loss}
  \end{subfigure}
  \caption{\textbf{Loss curve with/without satellite correction strategy.} The orange curves are the loss curves of SGFormer without the satellite correction, while blue curves are the loss curves with satellite correction.}
    \label{fig:loss}
\end{figure*}

\begin{table*}[htb]
\centering
\scalebox{1}{
\begin{tabular}{ccc|cccc}
\toprule
Channel Attention & Spatial Attention & Probability  Net & IoU     & mIoU    & Global   & Detail \\ \midrule
\ding{55}           & \ding{55}          & \ding{55}   & 43.90 & 15.59 & 28.43 & 8.10 \\
\ding{51}         &   \ding{55}     &    \ding{55}      & 44.85& 16.25  & 29.19 & 8.71\\
\ding{55}          &\ding{51}       &     \ding{55}     & 44.88& 16.12   & \bf{29.97} & 8.05\\
\ding{55}         &   \ding{55}      & \ding{51}        & 44.95 & 16.45& 29.06& 9.12 \\
\ding{51}          & \ding{51}        & \ding{51}        & \bf{45.01} & \bf{16.68} & 29.31& \bf{9.29}\\
\bottomrule
\end{tabular}}
\caption{Ablation on components of fusion module.}
\label{tab:ablation_ex_1}
\end{table*}

\begin{table}[ht]
        \centering
        \begin{tabular}{l|cc}
            \toprule
            Ground image backbone \  & IoU            & mIoU           \\
            \midrule
            ResNet-50            & 44.30          & 16.14        \\
            EfficientNet-B7           & \textbf{45.01} & \textbf{16.68} \\
            \bottomrule
        \end{tabular}
        \caption{Ablation on different backbones.}
        \label{tab:ablation_ex_2}
\end{table}

\section{Extended Technical Details}
\subsection{Convolutional Enhancement Details}
In the convolutional enhancement module, we utilize 3D and 2D U-Nets to improve prediction performance. For the ground branch, we employ a 3D U-Net with two encoder and decoder layers. In the satellite branch, we use a 2D U-Net with three encoder and decoder layers.
\subsection{Fusion Module Details}
Our channel and spatial attention mechanisms used in the dual-path weight generator are inspired by CBAM \cite{cbam}, with the detailed architecture illustrated in Figure~\ref{fig:attention}.

\noindent \textbf{Channel Attention.} The channel attention operation is shown in the upper part of Figure~\ref{fig:attention}. First, we compress the concatenated voxel features along the spatial dimensions using both average and maximum pooling operations, generating $\mathbf{F}_{channel}^{avg}$ and $\mathbf{F}_{channel}^{max}\in \mathbb{R}^{D \times 1 \times 1 \times 1}$. These compressed features are then passed through shared MLP layers consisting of two MLP layers with a ReLU activation function, producing two channel attention maps $\mathbf{W}_{c}^{avg}$ and $\mathbf{W}_{c}^{max}  \in \mathbb{R}^{D \times 1 \times 1 \times 1}$. Finally, we sum the two maps to compute the channel attention weight $\mathbf{W}_{c}$. Mathematically, the whole operation can be expressed as:
\begin{equation}
    \small
    \mathbf{W}_{c} = \operatorname{MLP}(\operatorname{AvgPool}(\mathbf{F'}_c^{3D})) + \operatorname{MLP}(\operatorname{MaxPool}(\mathbf{F'}_c^{3D}))
\end{equation}
where $\operatorname{MLP}$ is the shared MLP layers, $\operatorname{AvgPool}$ and $\operatorname{MaxPool}$ is average and maximum pooling operation, respectively. 

\noindent \textbf{Spatial Attention.} The spatial attention operation is shown in the lower part of Figure~\ref{fig:attention}. Similar to the channel attention operation, we compress the concatenated BEV features along the channel axis to obtain $\mathbf{F}_{spatial}^{avg}$ and $\mathbf{F}_{spatial}^{max} \in \mathbb{R}^{1 \times H \times W}$. These features are concatenated and fed into a convolutional layer with a $7 \times 7$ kernel, producing the spatial attention weight $\mathbf{W}_{s}$. The equation of the spatial attention operation is shown as follows:
\begin{equation}
    \mathbf{W}_{s} = \operatorname{conv^{7\times 7}}(\operatorname{AvgPool}(\mathbf{F'}_c^{BEV}) \textcircled{c} \operatorname{MaxPool}((\mathbf{F'}_c^{BEV})))
\end{equation}
where $\textcircled{c}$ is concatenate operation, while $\operatorname{conv^{7\times 7}}$ is convolution operation with the $7 \times 7$ kernel. 

Additionally, in our probability network, the spatial attention operation follows the same steps. However, since the input features are voxel features, the convolutional layer is replaced with a 3D dilated convolution. Moreover, the MLP used in the weight generator is a 2-layer MLP with ReLU activation. In the probability net, we utilize a basic ResNet block \cite{resnet} combined with a 2-layer MLP.

\subsection{Loss Function Detail}
\textbf{Scene Class Affinity Loss.} Our scene class affinity loss is the same as previous work~\cite{monoscene,voxformer}. The loss computes the class-wise derivable precision, recall, and specificity. The mathematical equation is:
\begin{equation}
\begin{aligned}
P_c(\hat{p}, p) & =\log \frac{\sum_i \hat{p}_{i, c}\left[p_i=c\right]}{\sum_i \hat{p}_{i, c}} \\
R_c(\hat{p}, p) & =\log \frac{\sum_i \hat{p}_{i, c}\left[p_i=c\right]}{\sum_i\left[p_i=c\right]} \\
S_c(\hat{p}, p) & =\log \frac{\sum_i\left(1-\hat{p}_{i, c}\right)\left(1-\left[p_i=c\right]\right)}{\sum_i\left(1-\left[p_i=c\right]\right)}
\end{aligned}
\end{equation}
where the $\hat{p}_{i, c}$ is the predicted probability for the class c, while $p_i$ is the ground truth. $P_c$ and $R_c$ denote the precision and recall, respectively, evaluating the performance of voxels belonging to class c. And $S_c$ is specificity, which measures the performance of voxels not belonging to class c. We get the scene class affinity loss $\mathcal{L}_{scal}$ by summing the $P_c$, $R_c$, and $S_c$ together as follows:
\begin{equation}
\mathcal{L}_{\text {scal }}(\hat{p}, p)=-\frac{1}{C} \sum_{c=1}^C\left(P_c(\hat{p}, p)+R_c(\hat{p}, p)+S_c(\hat{p}, p)\right) .
\end{equation}
In our paper, we use the semantic label and binary geometry label to obtain semantics affinity loss $\mathcal{L}_{\text {scal }}^{\text{sem}}$ and geometry affinity loss $\mathcal{L}_{\text {scal }}^{\text{geo}}$, respectively, and add them together.

\noindent \textbf{Cross-Entropy Loss.} As mentioned in Section 3.5 of the paper, we use weighted cross-entropy loss to compute three losses: $\mathcal{L}_{ce}$, $\mathcal{L}_{co}$, and $\mathcal{L}_{bev}$. Our cross-entropy equation is expressed as follows:
\begin{equation}
loss=-\sum_{c=1}^N w_c \log \frac{\exp \left(\hat{y}_{c}\right)}{\sum_{i=1}^N \exp \left(\hat{y}_{i}\right)} y_{c}
\end{equation}
where $\hat{y}$ is input, y is the ground truth, and N denotes the class number. $w_c$ is the class weight that is inverse of class frequency.
\section{Additional Ablation Study}
\label{sec:aablation}
In this section, we present the additional ablation analysis, which consists of three parts: adaptive fusion module, Backbone, and learning efficiency.  
\subsection{Ablation on Adaptive Fusion Module}
Table~\ref{tab:ablation_ex_1} presents the ablation on detailed components of our adaptive fusion module. Overall, the integration of any component within our fusion module significantly enhances the prediction accuracy of SGFormer. This improvement arises because the two branches focus on different aspects of the task; thus, introducing an adaptive weighting mechanism naturally brings substantial performance improvement. Specifically, incorporating the \textbf{channel attention network} simultaneously improves the accuracy for both scene layout and small objects: the mIoU for the "global" category increases from 28.43 to 29.19, while the mIoU for the "detail" category improves from 8.10 to 8.71. This enhancement is attributed to the module's capability to perform trade-offs at the object level, making the fusion strategy more inclined to rely on the satellite branch's outputs for objects in the "global" category and on the ground branch for the "detail" category.

The addition of the \textbf{spatial attention network} further increases the accuracy of our method in capturing the scene layout, increasing the mIoU from 28.43 to 29.97. This improvement is due to the spatial attention network's ability to balance the weights of the sensors across different regions based on each sensor's detection range, enabling our method to generate a more comprehensive scene layout.

Finally, the incorporation of the \textbf{probability net} enhances the prediction accuracy across all categories. The probability net adaptively identifies the more important voxels, thereby improving the overall learning efficiency of the model.

\subsection{Ablation on Image Backbone}
Table~\ref{tab:ablation_ex_2} shows the comparison between different ground image backbones, including EfficientNet-B7~\cite{efficientnet} (used in SGFormer) and ResNet-50~\cite{resnet} (used in baseline methods such as VoxFormer and Symphonize). The results highlight two key observations. First, EfficientNet-B7 achieves higher performance due to its more efficient architecture. Second, even when using ResNet-50, SGFormer still outperforms baseline methods, demonstrating the superiority of our dual-branch framework.

\subsection{Ablation on Learning Efficiency}
Figure~\ref{fig:loss} shows the learning curves of our method with and without satellite correction strategy. We report all the losses we used in the training, including BEV loss,  scene class affinity loss, and cross-entropy loss (summed with coarse loss). According to the figure, adding satellite correction operations can improve learning efficiency. This finding confirms what we mentioned about adding satellite correction to warm up learning. 
\section{Additional Visualization}
Figure~\ref{fig:vis_a1} and Figure~\ref{fig:vis_a2} presents the more visualization results from SemanticKITTI~\cite{semantickitti}. Moreover, we include qualitative results on the SSCBench-KITTI-360 dataset~\cite{sscbench}. Since VoxFormer~\cite{voxformer} does not provide code for SSCBench-KITTI-360, we only compare our method to Symphonize~\cite{symphonize} on this dataset. 
\section{Limitation}
Although our work has achieved excellent results on two datasets, it still has several limitations. First, our method relies on appropriate satellite map inputs, and previous ablation experiments have shown that our approach is quite sensitive to localization noise. Therefore, if there is a significant deviation between the input satellite imagery and the actual location, the performance of our method will be greatly reduced. Additionally, we have not introduced many innovations targeting dynamic and small objects; thus, for these categories, our method does not show significant improvements compared to other approaches. Finally, adding a satellite branch brings additional computational resource, making our method less lightweight. We will address these issues in future work. Despite the above problems, we still believe that our method has made a valuable contribution and provided inspiration to the field of SSC task.
%\mathcal{L}=\mathcal{L}_{s c a l}^{g e o}+\mathcal{L}_{\text {scal }}^{s e m}+\mathcal{L}_{c e} + \lambda_{bev}\mathcal{L}_{bev} + \lambda_{co}\mathcal{L}_{co},

\begin{figure*}
    \centering
    \includegraphics[width=\linewidth]{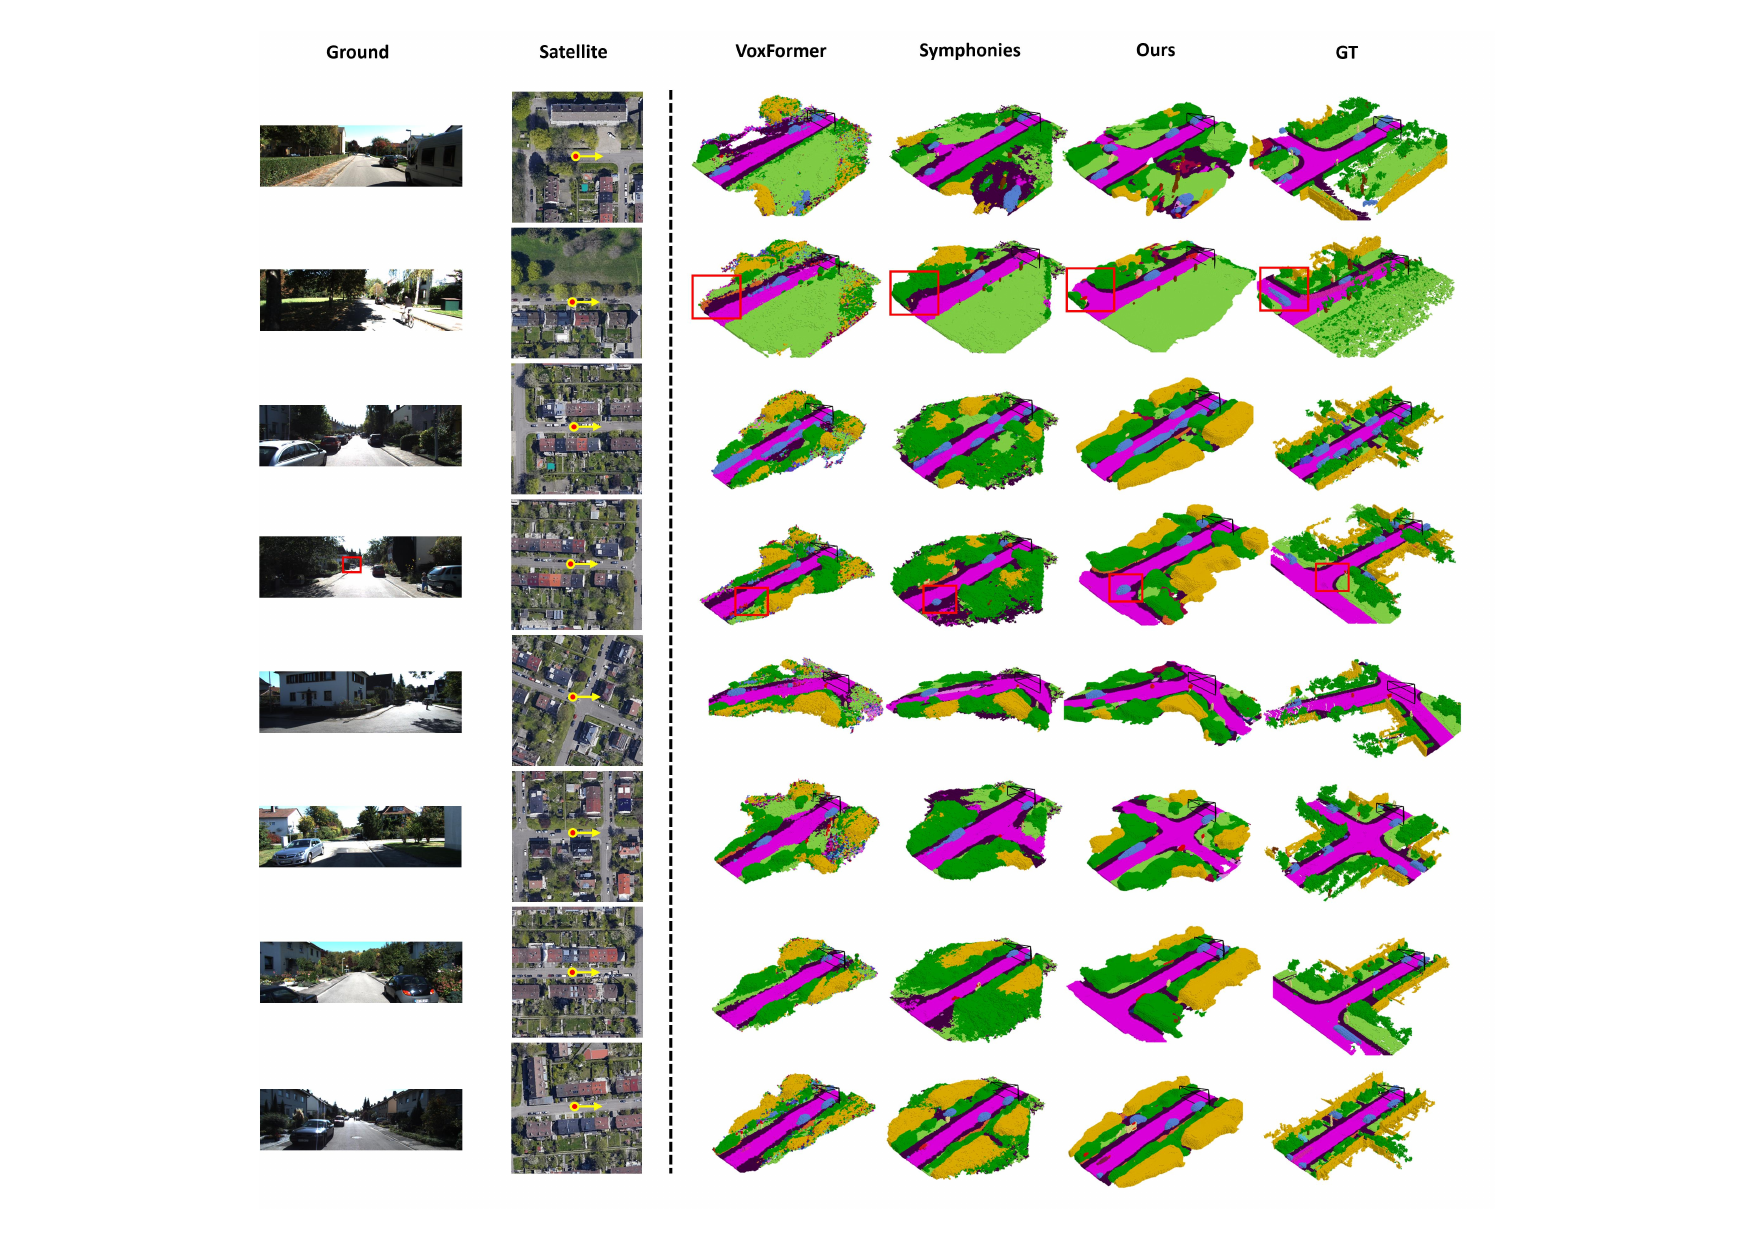}
    \caption{\textbf{Additional Visualization on SemanticKITTI~\cite{semantickitti}.}}
    \label{fig:vis_a1}
\end{figure*}

\begin{figure*}
    \centering
    \includegraphics[width=\linewidth]{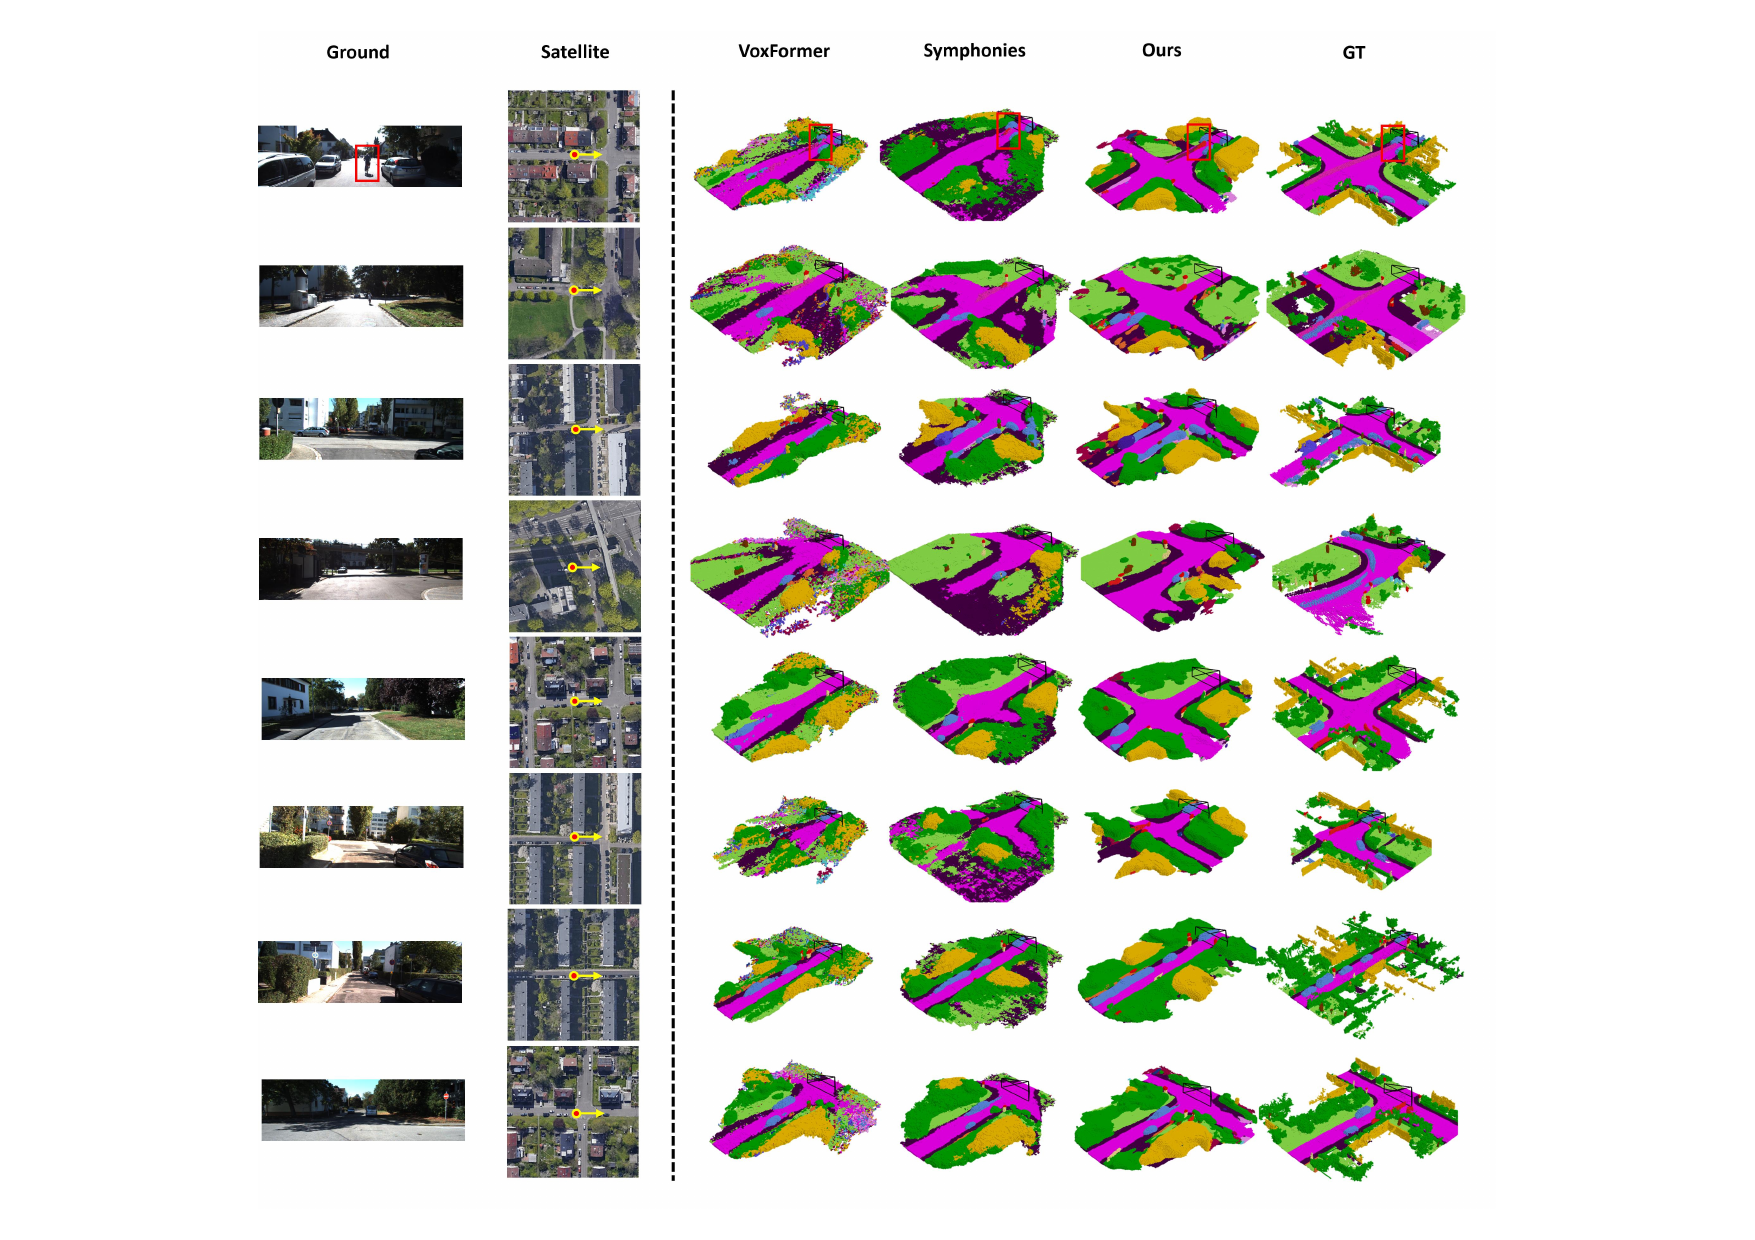}
    \caption{\textbf{Additional Visualization on SemanticKITTI~\cite{semantickitti}.}}
    \label{fig:vis_a2}
\end{figure*}

\begin{figure*}
    \centering
    \includegraphics[width = \linewidth]{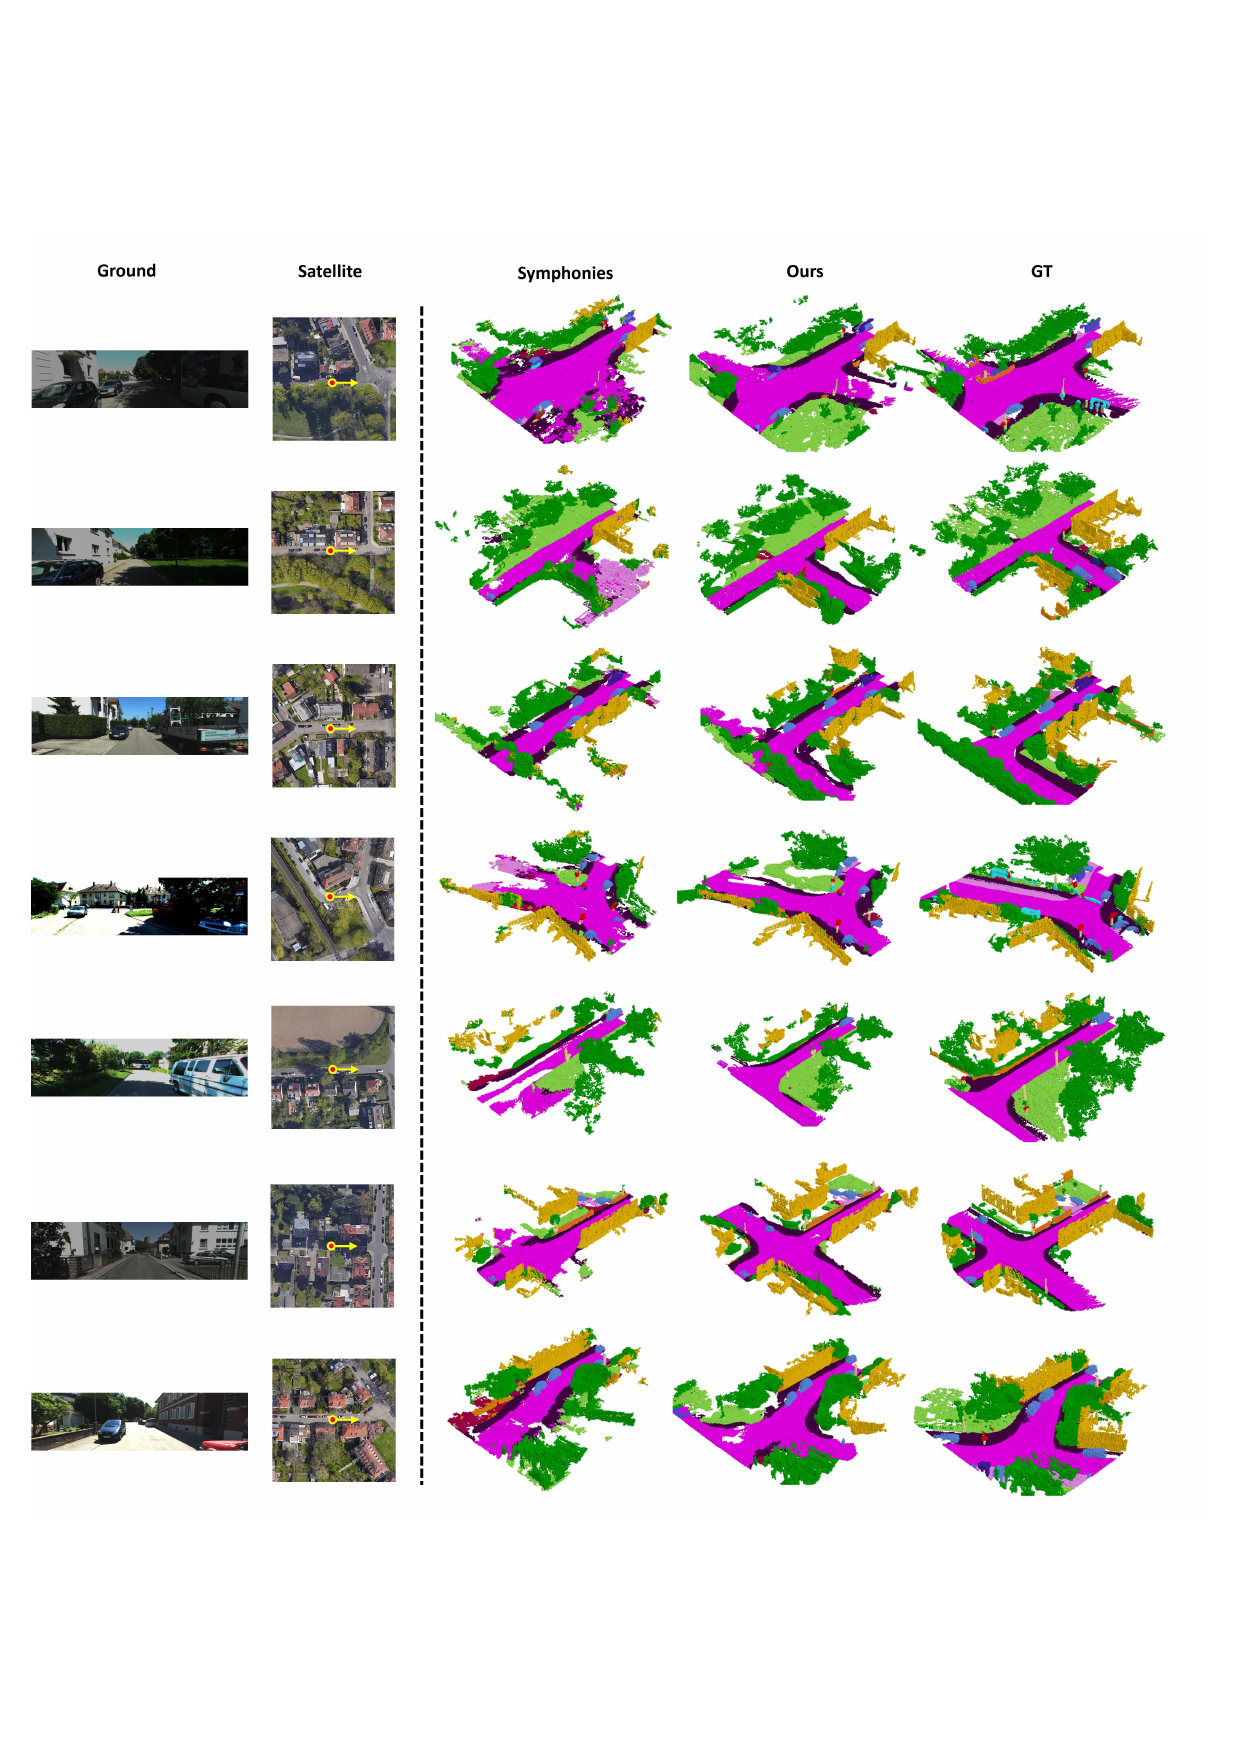}
    \caption{\textbf{Additional Visualization on SSCBench-KITTI-360~\cite{sscbench}.}}
    \label{fig:vis_a3}
\end{figure*}
